# Supplementary material for: Surface reconstruction of tetragonal methylammonium lead triiodide
Source: arXiv:2108.10523 source file (2021-08-24)
Supplement: Supplementary file 1 [file SM.tex]

\documentclass[notitlepage,prb,amssymb,amsmath,floatfix,superscriptaddress,aps,10pt]{revtex4-1}

\usepackage{graphicx}

\usepackage{bm}

\usepackage{lipsum}

%\usepackage{longtable}

\usepackage{threeparttable}

%% Language and font encodings
\usepackage[english]{babel}
\usepackage[utf8x]{inputenc}
\usepackage[T1]{fontenc}

%\usepackage{color}
\usepackage{graphics}
\usepackage{graphicx}
\usepackage{subfigure}
\usepackage{epsfig}
%\usepackage{subcaption} % Customize caption styles
%\usepackage{multicol}
\usepackage{etoolbox}
\usepackage{setspace}
\usepackage{nonfloat}
%\usepackage{a4wide}
%\usepackage{caption}
% Page Layout Packages
\usepackage{lastpage} % Get access to the number of pages
%\usepackage{fancyhdr}
%\usepackage{wrapfig}  % Another package for wrapping text - just for figures
\usepackage{appendix}
\renewcommand\abstractname{\textit{Abstract}}
%\usepackage{float}
\usepackage{parskip} % remove indentation from new paragraphs
\sloppy % Be less fussy about spacing, and avoid overfull boxes
\raggedbottom % Do not add extra vspace to fill page - bunch all at top
%% Useful packages
\usepackage{amsmath}
\usepackage[colorinlistoftodos]{todonotes}
\usepackage{hyperref}
%\usepackage[colorlinks=true, allcolors=black]{hyperref}
\usepackage{hhline}
\usepackage[Euler]{upgreek}
%\hypersetup{hidelinks=true}

%\pagestyle{fancy}
%%\Header/footer contents
%%\lhead{\small \sc Rinke} \chead{\small \sc Acronym} %\rhead{\small \sc Part B Section 1d (B1)}
%\lhead{} \chead{\small Coating hybrid perovskites: A database-driven study} 
%%\lfoot{} \cfoot{Page \thepage\ of \pageref{LastPage}} %\rfoot{}
%%\cfoot{\thepage\ of {\hypersetup{linkcolor=black}%\pageref{LastPage}}}

\addto\captionsenglish{\renewcommand{\figurename}{FIG.}}
\addto\captionsenglish{\renewcommand{\tablename}{TABLE}}

\renewcommand{\thesection}{S\arabic{section}}
\renewcommand{\thefigure}{S\arabic{figure}}
\renewcommand{\thetable}{S\arabic{table}}
%\addto\captionsenglish{\renewcommand{\figurename}{SM}}
%\addto\captionsenglish{\renewcommand{\tablename}{SM TABLE}}
%\renewcommand{\figurename}{SM FIG.} 
%\usepackage{cite}
%\newcommand{\JL}[1]{{\color{red}{#1}}}
\definecolor{aaltoOrange}{RGB}{255,121,0}%

\usepackage{xr}
%\usepackage{cleveref}
%\graphicspath{{../FitData}}
%\externaldocument{main}

\makeatletter
\newcommand*{\addFileDependency}[1]{% argument=file name and extension
  \typeout{(#1)}
  \@addtofilelist{#1}
  \IfFileExists{#1}{}{\typeout{No file #1.}}
}
\makeatother

\newcommand*{\myexternaldocument}[1]{%
    \externaldocument{#1}%
    \addFileDependency{#1.tex}%
    \addFileDependency{#1.aux}%
}

\myexternaldocument{main}
\newcommand{\PRc}[1]{\textcolor{aaltoOrange}{{\bf PR: #1 }}}

\usepackage{soul}
%\addto\captionsenglish{\renewcommand{\figurename}{S\english{FIG.}}}
%\addto\captionsenglish{\renewcommand{\tablename}{TABLE}}
\newcommand{\JL}[1]{{\color{red}{#1}}}
%\newcommand{\JL}[1]{{\color{black}{#1}}}
\newcommand{\JLc}[1]{{\color{cyan}{\textbf{(JL: #1)}}}}
\newcommand{\JLst}[1]{{\color{gray!50}{\st{#1}}}}

\begin{document} 

\title%[$\text{CsPbI}_3$ surface modeling]
{{\normalsize{Supplementary Material for}} \\ ~ \\ Surface reconstruction of tetragonal methylammonium lead triiodide}

\author{Azimatu Seidu}
\affiliation{Department of Applied Physics, Aalto University, FI-00076 AALTO, Finland}
\author{Marc Dvorak}
\affiliation{Department of Applied Physics, Aalto University, FI-00076 AALTO, Finland}
\author{Jari J\"arvi}
\affiliation{Department of Applied Physics, Aalto University, FI-00076 AALTO, Finland}
\author{Patrick Rinke}
\affiliation{Department of Applied Physics, Aalto University, FI-00076 AALTO, Finland}
\author{Jingrui Li}
\affiliation{Electronic Materials Research Laboratory, Key Laboratory of the Ministry of Education \& International Center for Dielectric Research, School of Electronic Science and Engineering, Xi'an Jiaotong University, Xi'an 710049, China}
%\altaffiliation[Also at ]{Department of Applied Physics, Aalto University, P.O.Box 11100, FI-00076 AALTO, Finland} %Lines break automatically or can be forced with \\
%\email{jingrui.li@aalto.fi}

\maketitle
\section{Surface phase diagrams of $\text{PbI}_2^{}$\,-T surface models}

Figure~\ref{stds_pbi2} depicts the surface phase diagrams of PbI$_2$-T surface models. The yellow regions show the thermodynamically stable limit for the growth of bulk $\text{MAPbI}_3^{}$\,. 

\begin{figure}[!htp]
\centering
\includegraphics[width=\linewidth]{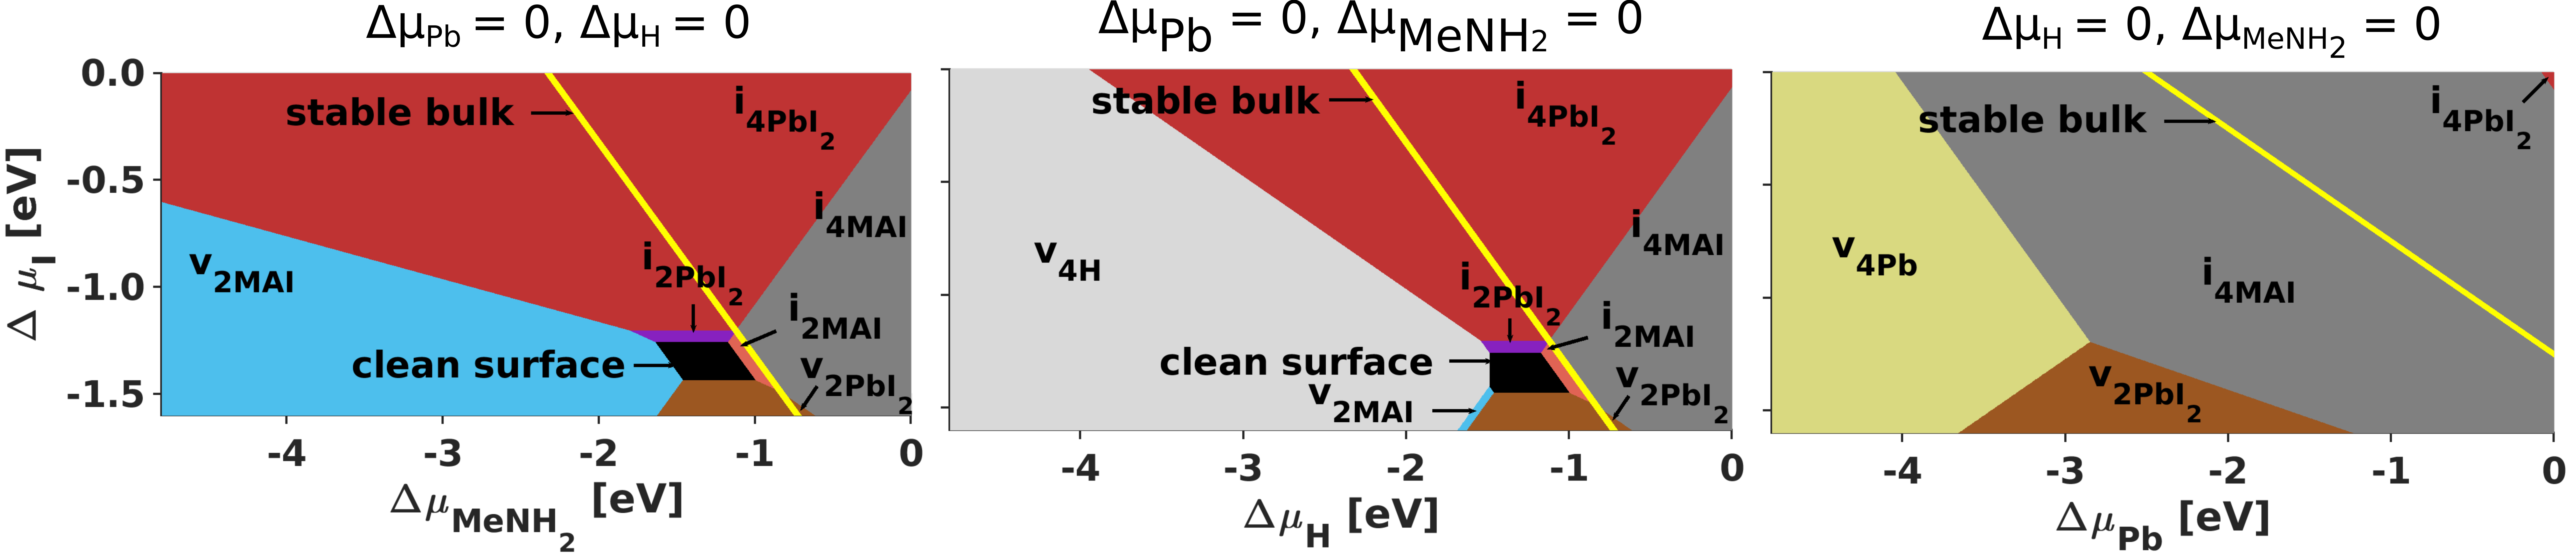}
\caption{Surface phase diagrams of reconstructed PbI$_2$\,-T surface models of tetragonal MAPbI$_3$\,. The yellow regions depict the thermodynamically stable range for the growth of bulk $\text{MAPbI}_3^{}$\,.} \label{stds_pbi2} 
\end{figure}

\newpage
\section{Most relevant optimised reconstructed PbI$_{2}$\,-T surface models }

Figure~\ref{struct_pbi2} depicts the optimized structures of the most relevant reconstructed PbI$_2$\,-T surface models. The top panel shows the top view of the topmost atoms with the light gray shades, depicting the topmost octahedra.

\begin{figure}[!htp]
\includegraphics[width=\linewidth]{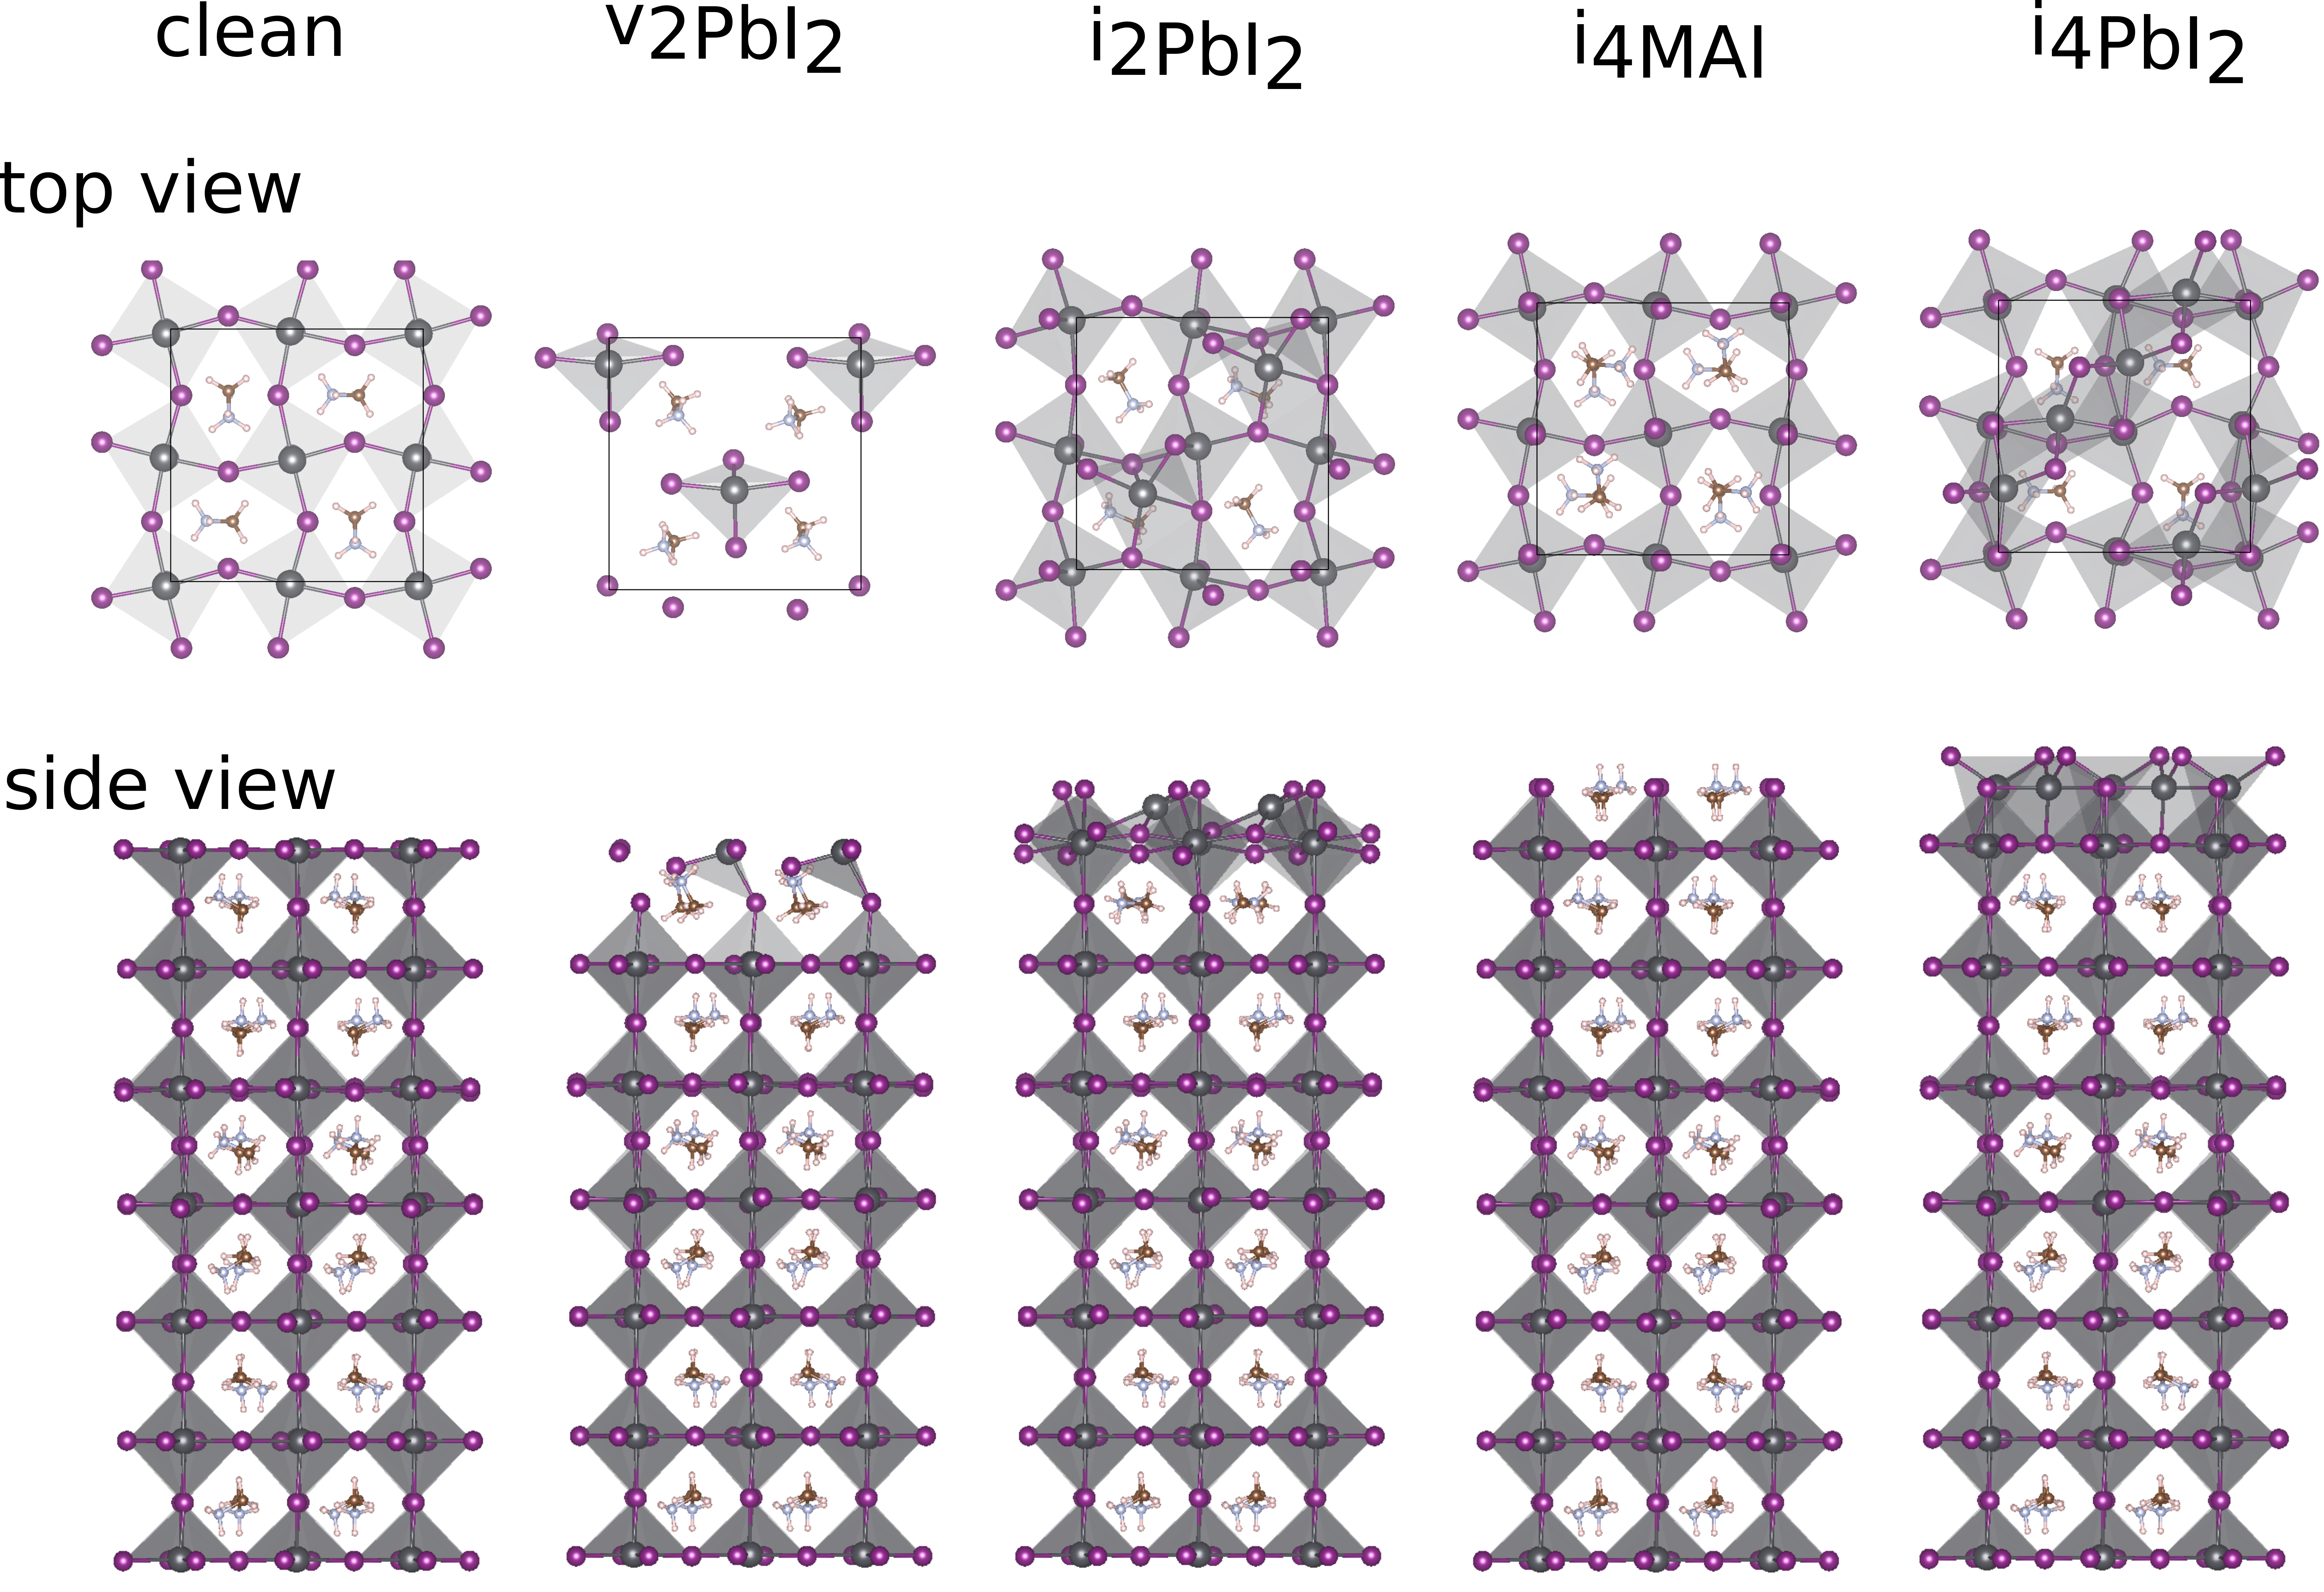}
\caption{Optimized crystal structures the most relevant recontruvted PbI$_2$\,-T surface models of tetragonal MAPbI$_3$\,. } \label{struct_pbi2} 
\end{figure}


\newpage
\section{Band structure of the most relevant reconstructed surface models with PbI$_2$\,-T}
Band structures of the most relevant reconstructured surface model with PbI$_2$-terminations are shown in Fig.~\ref{bands_pbi2}. The valence band maximum is set to zero and depicted with the red line. The projected bulk band structures is included as blue shading for comparison.  

\begin{figure}[!htp]
\includegraphics[width=0.8\linewidth]{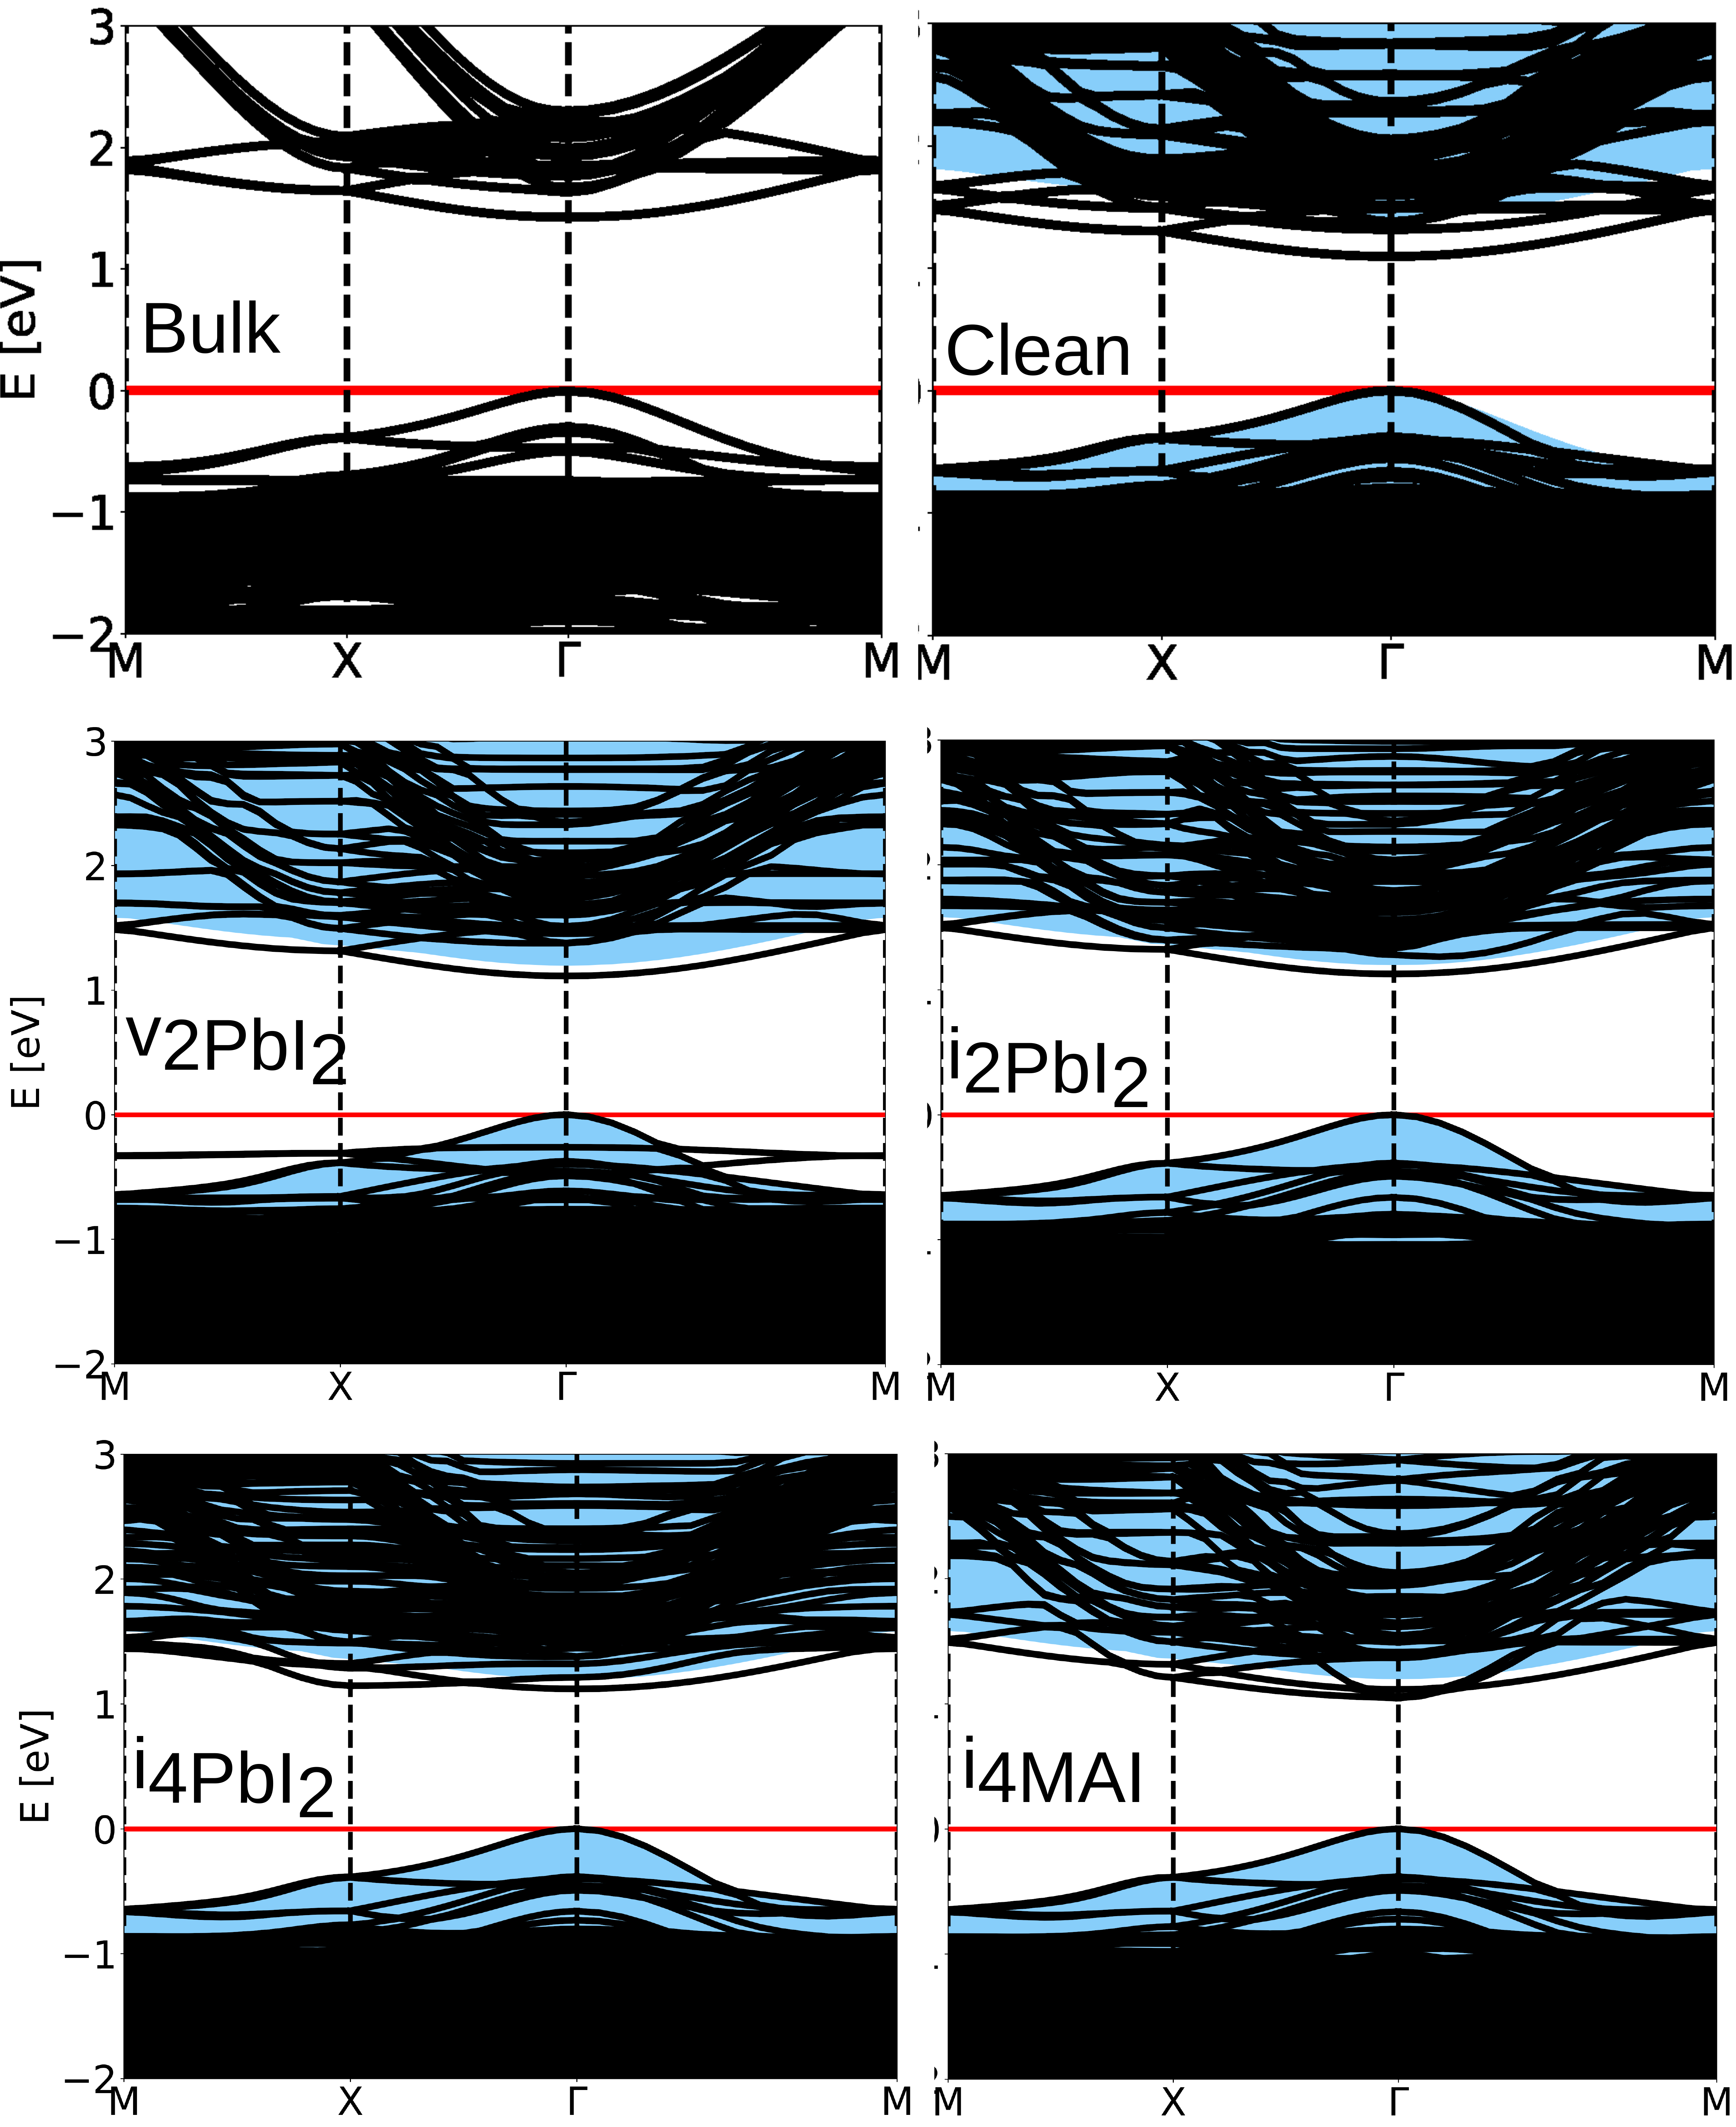}\vspace{-.5em}
\caption{Band structures of bulk and the most relevant reconstructed  PbI$_2$\,-T surface models of  MAPbI$_3$.  In the surface band structure plots, the projected bulk band structure is shown as blue shading. The red line depicts the valence band maximum (VBM).}\label{bands_pbi2}
\end{figure}

\end{document}
